# Supplementary material for: Context-aware Domain Adaptation for Time Series Anomaly Detection
Source: arXiv:2304.07453 source file (2023-04-15)
Supplement: Supplementary file 1 [file supplementary.tex]

\usepackage[letterpaper]{geometry}

\usepackage{ltexpprt}
\usepackage{hyperref}

%%%%%%%%%%%%%%%%%%%%%%%%%
\usepackage{subcaption}
\usepackage{diagbox}
\usepackage{multirow}
\usepackage{multicol}
\usepackage{algorithm}
\usepackage{enumitem}
\usepackage{algorithmic}
\usepackage{booktabs}
\usepackage{graphicx}
\usepackage{subfigure}
%%%%%%%%%%%%%%%%%%%%%%%%%

\begin{document}

\end{document}
